# Supplementary material for: Beamforming Cancellation Design for Millimeter-Wave Full-Duplex
Source: arXiv:1908.06505 source file (2020-06-30)
Supplement: Supplementary file 1 [file eq-si-channel-nlos.tex]

\begin{align} \label{eq:si-channel-nlos}
	\channel^{\textrm{NLOS}}_{i,i} &= 
\end{align}
