# Supplementary material for: Beamforming Cancellation Design for Millimeter-Wave Full-Duplex
Source: arXiv:1908.06505 source file (2020-06-30)
Supplement: Supplementary file 2 [file eq-si-channel.tex]

\begin{align}
	\channel_{i,i} &= \sqrt{\frac{\kappa}{\kappa + 1}} \channel^{\textrm{LOS}}_{i,i} + \sqrt{\frac{1}{\kappa + 1}} \channel^{\textrm{NLOS}}_{i,i}
\end{align}
